# Supplementary material for: StylePart: Image-based Shape Part Manipulation
Source: arXiv:2111.10520 source file (2022-04-07)
Supplement: Supplementary file 1 [file cgf_supp_metadata.tex]

\title[Supplemental Material for StylePart: Image-based Shape Part Manipulation]%
      {Supplemental Material for StylePart: Image-based Shape Part Manipulation}

\author[paper1003]{paper1003}
